# Supplementary material for: Defending against Machine Learning based Inference Attacks via Adversarial Examples: Opportunities and Challenges
Source: arXiv:1909.08526 source file (2019-09-19)
Supplement: Supplementary file 1 [file appendix.tex]

\section*{Appendix}
\addcontentsline{toc}{section}{Appendix}
%\appendices
\section{Game-Theoretic Formulation}
\label{gametheory}
Shokri et al.~\cite{ShokriCCS12} proposed a game-theoretic formulation for defending against location inference attacks. In location inference attacks, both the public data and private attribute are users' true locations. Specifically, a user's true public data is the user's true location; the defender obfuscates the true location to a fake location; and the attacker aims to infer the user's true location, which can also be viewed as the user's private attribute. The game-theoretic formulation defends against the optimal location inference attack that adapts based on the knowledge of the defense. We extend this game-theoretic formulation for attribute inference attacks. In attribute inference attacks, public data and private attributes are different. 

%The location is discretized

%We show details about Bayesian formulation to protect private attributes from being inferred by public data. 
%We note that this Bayesian formulation is not our contribution and was adapted from the one proposed by Shokri et al.~\cite{ShokriCCS12} and Calmon et al.~\cite{Calmon:2012}. 
%We describe the details in order to demonstrate why Bayesian formulation makes the problem computationally intractable. 

\subsection{Notations} 
\addcontentsline{toc}{subsection}{Notations}
We denote by $s$ and $\mathbf{x}$ the private attribute and public data, respectively. 
We denote by $\text{Pr}(s,\mathbf{x})$ the joint probability distribution of  $s$ and $\mathbf{x}$. %Moreover, we use $\text{Pr}(\mathbf{x})$ and $\text{Pr}(s)$ to denote the marginal probability distributions of users' public data and private attribute, respectively.  %$P_{\mathbf{x}}(\mathbf{x}=\mathbf{x}_{0})$ is the probability that a randomly picked user has a public vector $\mathbf{x}_{0}$. Similarly, we denote by $P_s$ the marginal distribution of private attribute. %Thus, we have conditional probability distribution $P(s|\mathbf{x})=\frac{P_{s,\mathbf{x}}(s,\mathbf{x})}{P_{\mathbf{x}}(\mathbf{x})}$. 
The defender aims to find a probabilistic mapping $f$, which obfuscates a true public data $\mathbf{x}$ to a noisy public data $\mathbf{x}^\prime$ with a probability $f(\mathbf{x}^\prime|\mathbf{x})$. The probabilistic mapping $f$ is essentially a matrix, whose number of rows and number of columns is the domain size of the public data vector $\mathbf{x}$. 
%The defender knows the joint probability distribution $\text{Pr}(s,\mathbf{x})$ and aims to find a probabilistic mapping $f$
%The attacker knows $P_{s,\mathbf{x}}$, $f(\mathbf{x}^\prime|\mathbf{x})$, and $\mathbf{x}^\prime$, and aims to infer $s$. 

\subsection{Privacy Loss}
Suppose a user's true private attribute value is $s$ and an attacker infers the user's private attribute value to be $\hat{s}$. We denote the privacy loss for the user as a certain metric $d_p(s,\hat{s})$. 
%For a user, we define a user's privacy loss as a certain distance between the user true private attribute $s$ and attribute $\hat{s}$ inferred by attacker using noisy public data, i.e., $d_p(s,\hat{s})$. 
For example, one choice for the privacy loss metric could be:
\begin{align}
d_p(s,\hat{s})=
\begin{cases}
1 &\text{ if } s=\hat{s} \\
0 &\text{ otherwise,}
\end{cases}
\end{align}
which means that the privacy loss is 1 if the attacker correctly infers the user's attribute value, and 0 otherwise.

\subsection{Utility Loss} 
For a true public data vector $\mathbf{x}$ and its corresponding noisy vector $\mathbf{x}^\prime$, we define the utility loss as $d_q(\mathbf{x},\mathbf{x}^\prime)$, which could be any distance metric over $\mathbf{x}$ and $\mathbf{x}^\prime$. For instance, $d_q(\mathbf{x},\mathbf{x}^\prime)$ could be the $L_0$ norm of the noise $||\mathbf{x}^\prime-\mathbf{x}||_0$, which is the number of entries of $\mathbf{x}$ that are modified. Given the marginal probability distribution $\text{Pr}(\mathbf{x})$ and the probabilistic mapping $f$, we have the expected utility loss as follows:
\begin{align}
L=\sum_{\mathbf{x},\mathbf{x}^\prime}\text{Pr}(\mathbf{x}) f(\mathbf{x}^\prime|\mathbf{x})d_q(\mathbf{x}^\prime,\mathbf{x}).
\end{align}

\subsection{Defender's Strategy}
The defender aims to construct a probabilistic mapping $f$ to defend against the optimal inference attack subject to a utility-loss budget $\beta$. 
%
%\myparatight{Step 0} Randomly sample a private attribute value $s$ from the probability distribution $P_{s}$ and a true public data vector $\mathbf{x}$ from the probability distribution $P_{\mathbf{x}|s}$. 
%
%\myparatight{Step 1} Given $\mathbf{x}$, the defender runs $f(\mathbf{x}^\prime|\mathbf{x})$ to generate a noisy public data vector $\mathbf{x}^\prime$. 
%
%\myparatight{Step 2} After observing $\mathbf{x}^\prime$, the attacker performs a Bayesian inference attack to infer the private attribute value $\hat{s}=\argmax_s P(s|\mathbf{x}^\prime)$. 
The attacker knows the joint probability distribution $\text{Pr}(s,\mathbf{x})$ and the probabilistic mapping $f$. 
After observing a noisy public data vector $\mathbf{x}^\prime$, the attacker can compute a posterior probability distribution of the private attribute $s$ as follows:
\begin{align}
\text{Pr}(s|\mathbf{x}^\prime)&=\frac{\text{Pr}(s,\mathbf{x}^\prime)}{\text{Pr}(\mathbf{x}^\prime)} \\
&=\frac{\sum_{\mathbf{x}}\text{Pr}(s,\mathbf{x})f(\mathbf{x}^\prime|\mathbf{x})}{\text{Pr}(\mathbf{x}^\prime)}
%&=\frac{\sum_{\mathbf{x}}f(\mathbf{x}^\prime|\mathbf{x})\text{Pr}{s,\mathbf{x}}(s,\mathbf{x})}{\sum_{\mathbf{x}}\text{Pr}{\mathbf{x}}(\mathbf{x})f(\mathbf{x}^\prime|\mathbf{x})}
%&=\frac{f(\mathbf{x}^\prime|\mathbf{x})P_{\mathbf{x}}(\mathbf{x})}{\sum_{\mathbf{x}}f(\mathbf{x}^\prime|\mathbf{x})P_{\mathbf{x}}(\mathbf{x})}
\end{align}
Suppose the attacker infers the private attribute to be $\hat{s}$. Then, the conditional expected privacy loss is $\sum_{s}\text{Pr}(s|\mathbf{x}^\prime)d_p(s,\hat{s})$. 
%\begin{align}
%\sum_{s}\text{Pr}(s|\mathbf{x}^\prime)d_p(s,\hat{s}).
%\end{align}
Therefore, the maximum conditional expected privacy loss is as follows:
\begin{align}
\max_{\hat{s}}\sum_{s}\text{Pr}(s|\mathbf{x}^\prime)d_p(s,\hat{s})
\end{align}
%This posterior probability distribution represents the 
%Basically, the attacker aim to find user's private attribute $s$ to such that users' conditional average privacy loss is maximized and it can be expressed as follows: 
%\begin{align}
%\max_{s}d_q(P(s|\mathbf{x}),P(s|\mathbf{x}^\prime))
%\end{align}
Considering the probability distribution of $\mathbf{x}^\prime$, we have the unconditional expected privacy loss as follows:
\begin{align}
&\sum_{\mathbf{x}^\prime}\text{Pr}(\mathbf{x}^\prime)\max_{\hat{s}}\sum_{s}\text{Pr}(s|\mathbf{x}^\prime)d_p(s,\hat{s})\nonumber \\
=&\sum_{\mathbf{x}^\prime}\max_{\hat{s}}\sum_s\sum_{\mathbf{x}}\text{Pr}(s, \mathbf{x})f(\mathbf{x}^\prime|\mathbf{x})d_p(s,\hat{s}).
\end{align}
We define $y_{\mathbf{x}^\prime}=\max_{\hat{s}}\sum_s\sum_{\mathbf{x}}\text{Pr}(s, \mathbf{x})f(\mathbf{x}^\prime|\mathbf{x})d_p(s,\hat{s})$. The defender's goal is to minimize the unconditional expected privacy loss subject to a utility-loss budget. Formally, the defender aims to solve the following optimization problem:
\begin{align}
&\min \sum_{\mathbf{x}^\prime} y_{\mathbf{x}^\prime} \\
\text{subject to } &L \leq \beta.
\end{align}
According to Shokri et al.~\cite{ShokriCCS12}, this optimization problem can be transformed to the following linear programming problem: 
\begin{align}
&\min \sum_{\mathbf{x}^\prime} y_{\mathbf{x}^\prime} \nonumber \\
\text{subject to } &L \leq \beta \nonumber\\
& y_{\mathbf{x}^\prime} \geq \sum_s\sum_{\mathbf{x}}\text{Pr}(s, \mathbf{x})f(\mathbf{x}^\prime|\mathbf{x})d_p(s,\hat{s}), \forall \mathbf{x}^\prime, \hat{s} \nonumber\\
& \sum_{\mathbf{x}^\prime}f(\mathbf{x}^\prime|\mathbf{x}) = 1, \forall \mathbf{x} \nonumber\\
\label{gametheoryformulation}
& f(\mathbf{x}^\prime|\mathbf{x}) \geq 0, \forall \mathbf{x}, \mathbf{x}^\prime
\end{align}

\subsection{Limitations}
The formulated optimization problem is computationally intractable for attribute inference attacks in practice. Specifically, the computation cost is \emph{exponential} to the dimensionality of the public data vector, which is often high in practice. For instance, in recommender systems, a public data vector consists of a user's rating scores to the items that the user rated and 0 for the items that the user did not rate. Suppose a recommender system has 100 items (this is a very small recommender system in practice) and a rating score can be 1, 2, 3, 4, or 5. Then, the domain size of the public data vector $\mathbf{x}$ is $6^{100}$ and the size of the probabilistic mapping matrix $f$ is $6^{100} \times 6^{100}=6^{200}$. Therefore, even in the context of a very small recommender system with 100 items, it is intractable to solve the formulated optimization problem. 
